# Supplementary material for: Enhancing Ecological Monitoring with Multi-Objective Optimization: A Novel Dataset and Methodology for Segmentation Algorithms
Source: arXiv:2408.06356 source file (2024-07-25)
Supplement: Supplementary file 1 [file supp.tex]

\clearpage
\setcounter{page}{1}
\maketitlesupplementary

\section*{Supplementary Materials}
\setcounter{section}{0}

This supplementary document provides additional details on the data collection process, flight parameters, annotation artifacts, and more, complementing the main text of our paper. The following sections offer deeper insights into our methodology and the challenges encountered during the study.

\section{Research Team in Action}
Figure~\ref{fig:team_action} showcases images depicting the research team utilizing drone technology to capture a diverse array of indigenous and invasive grass species in the Bega Valley, New South Wales, Australia. These field activities highlight the practical aspects of our data collection efforts, emphasizing the meticulous planning and execution required to gather high-quality imagery under varying environmental conditions.

\begin{figure}[h!]
  \centering
  \begin{subfigure}[b]{0.23\textwidth}
    \includegraphics[width=\textwidth]{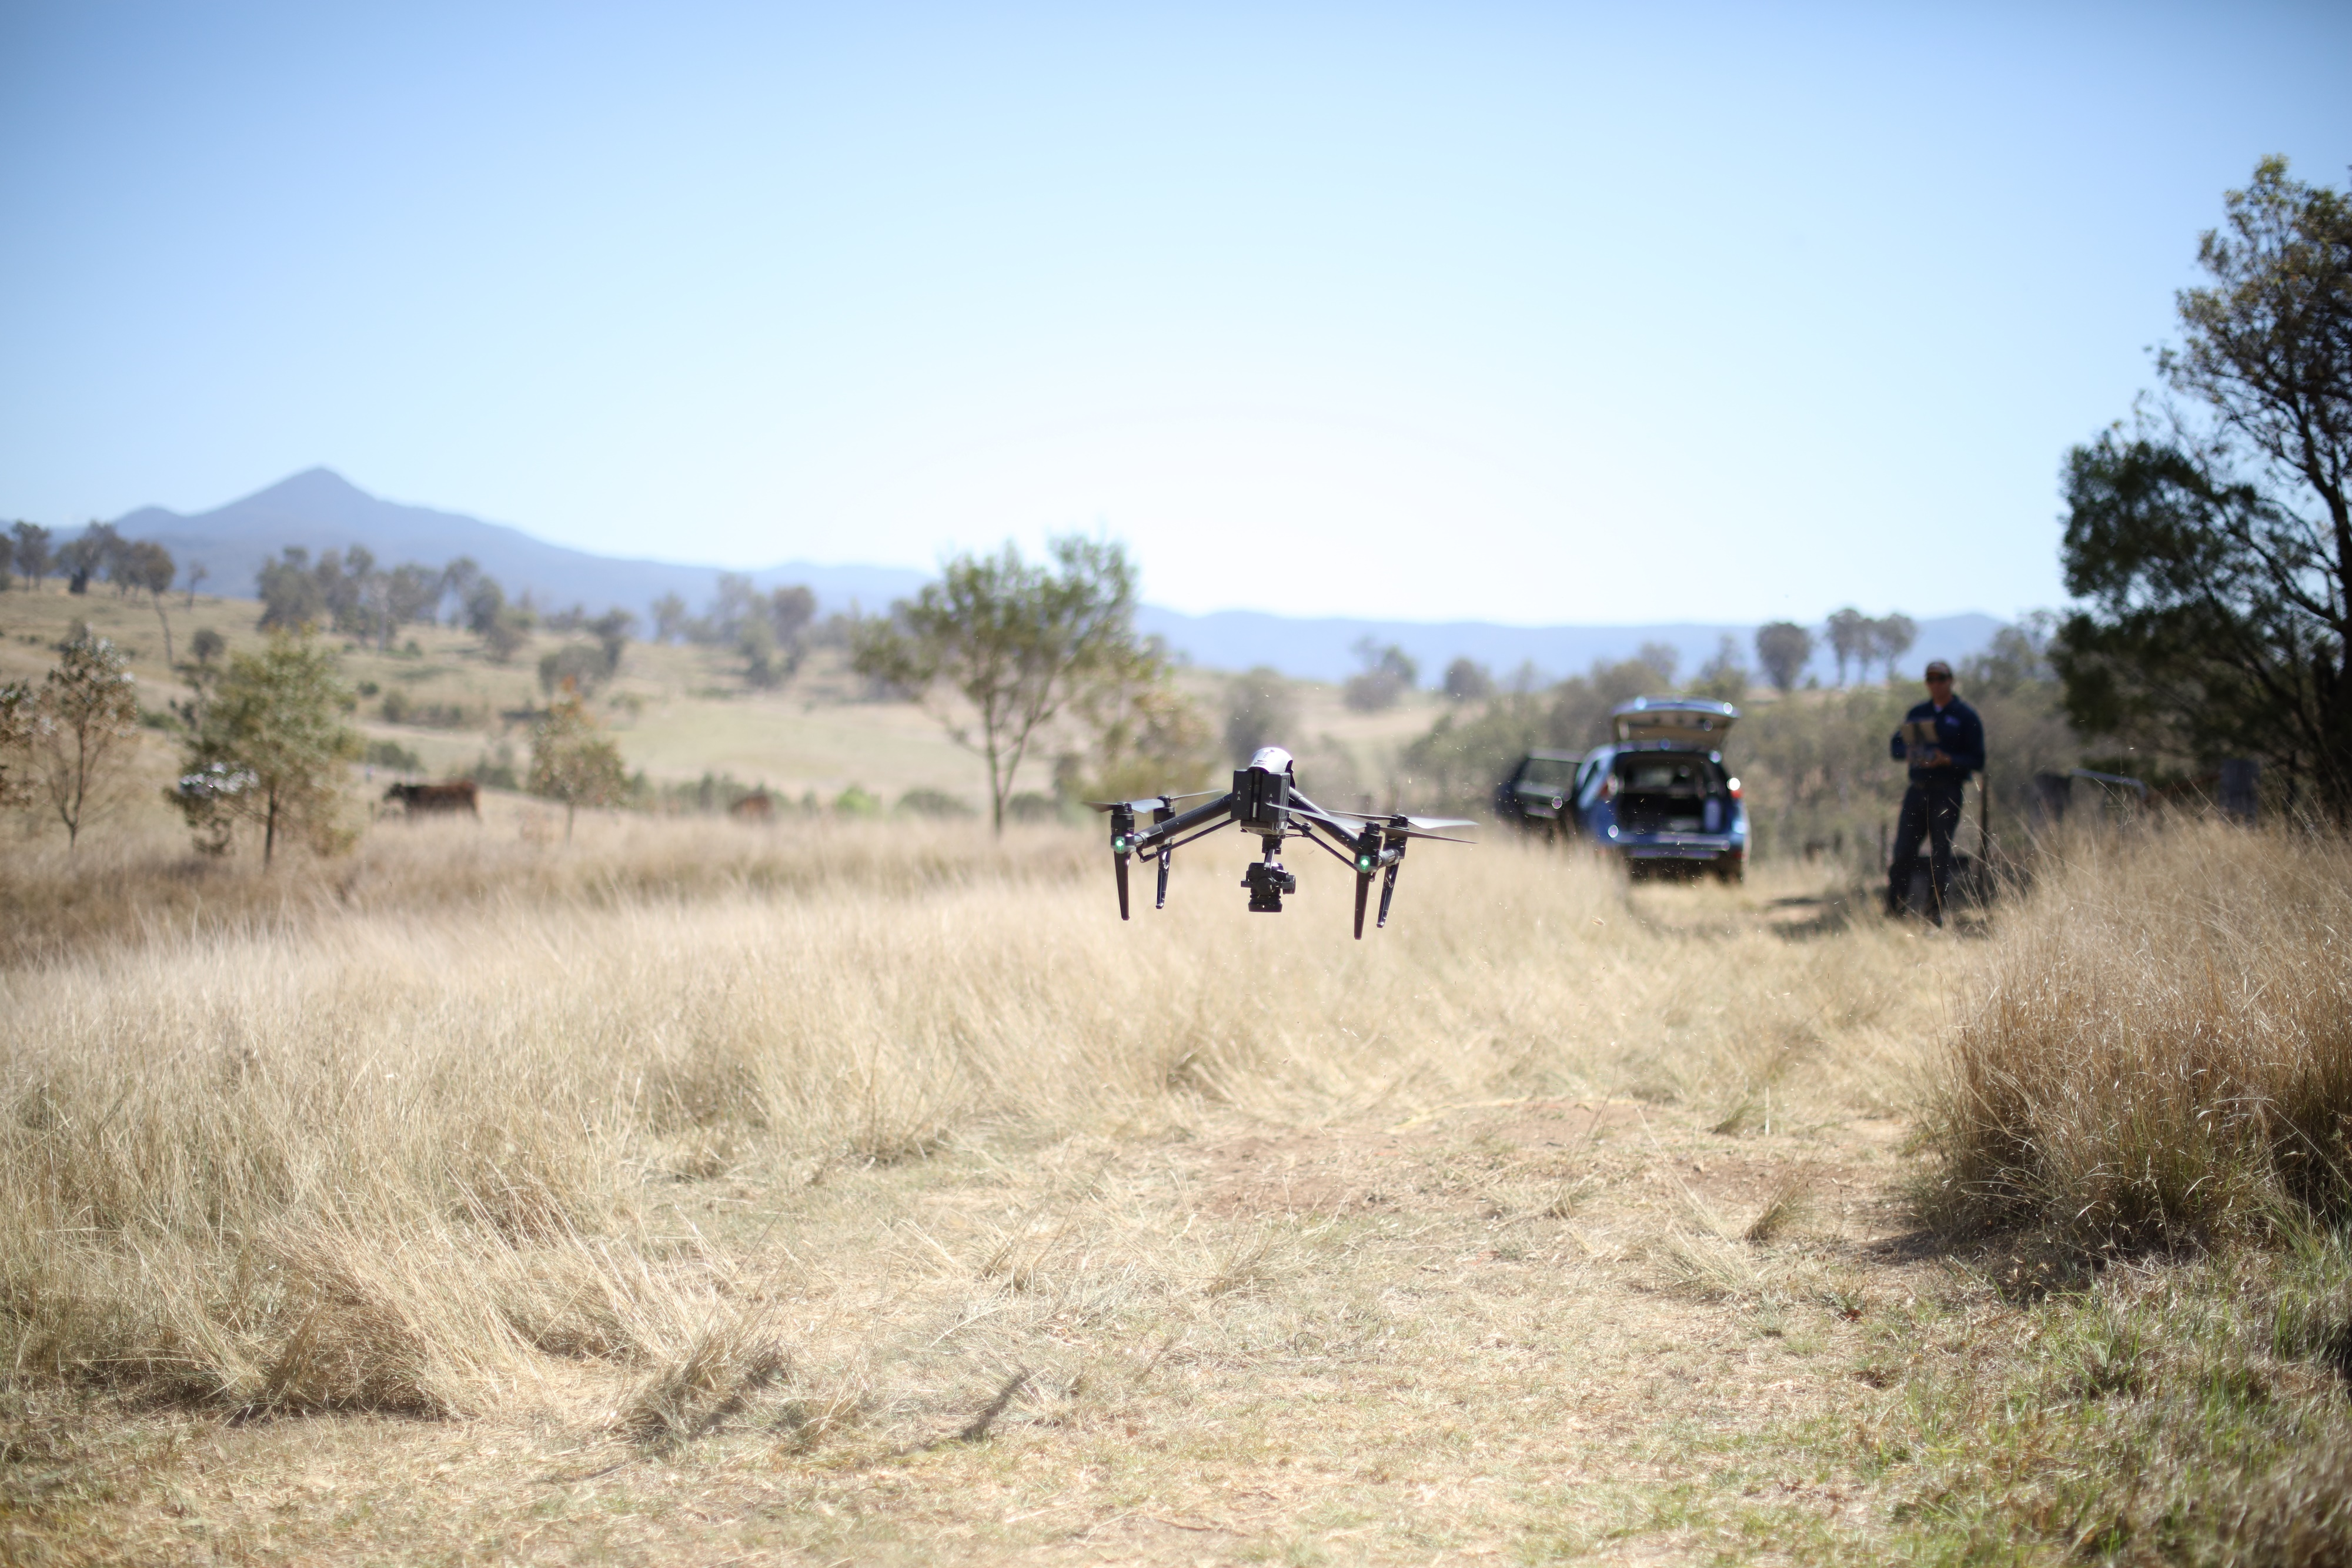}
    \label{fig:image1}
  \end{subfigure}
  \hfill
  \begin{subfigure}[b]{0.23\textwidth}
    \includegraphics[width=\textwidth]{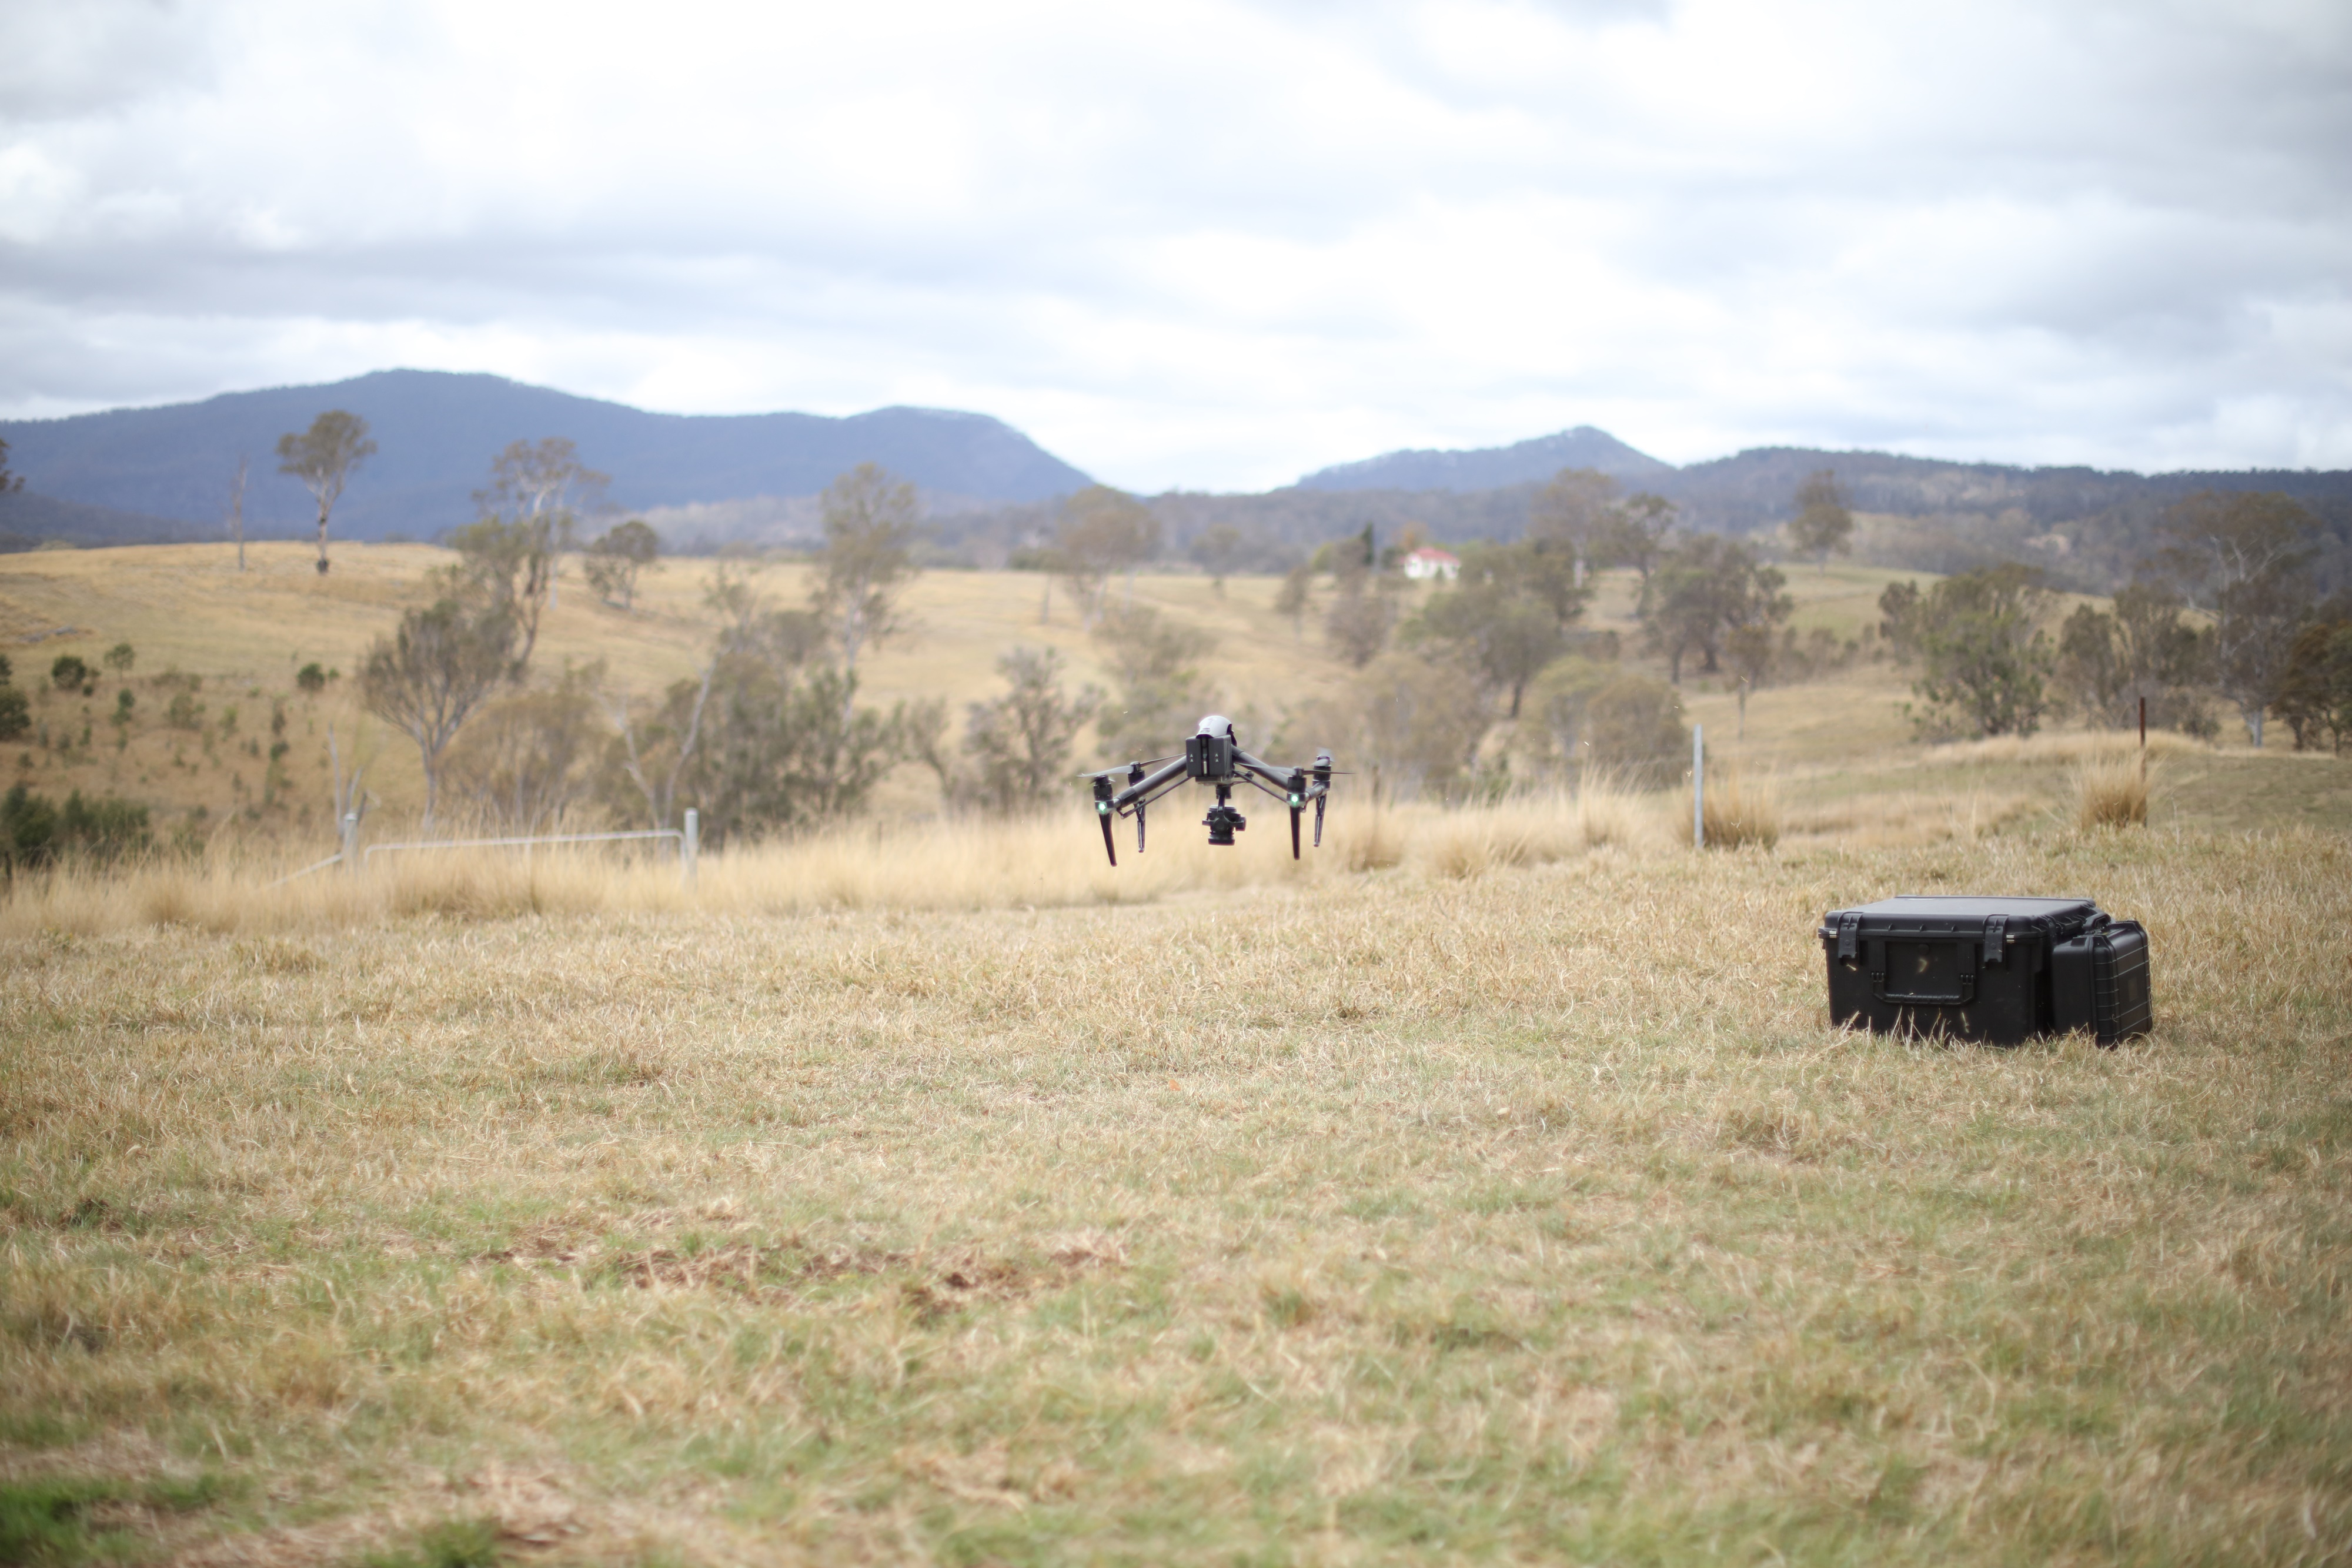}
    \label{fig:image2}
  \end{subfigure}
  \hfill
  \begin{subfigure}[b]{0.23\textwidth}
    \includegraphics[width=\textwidth]{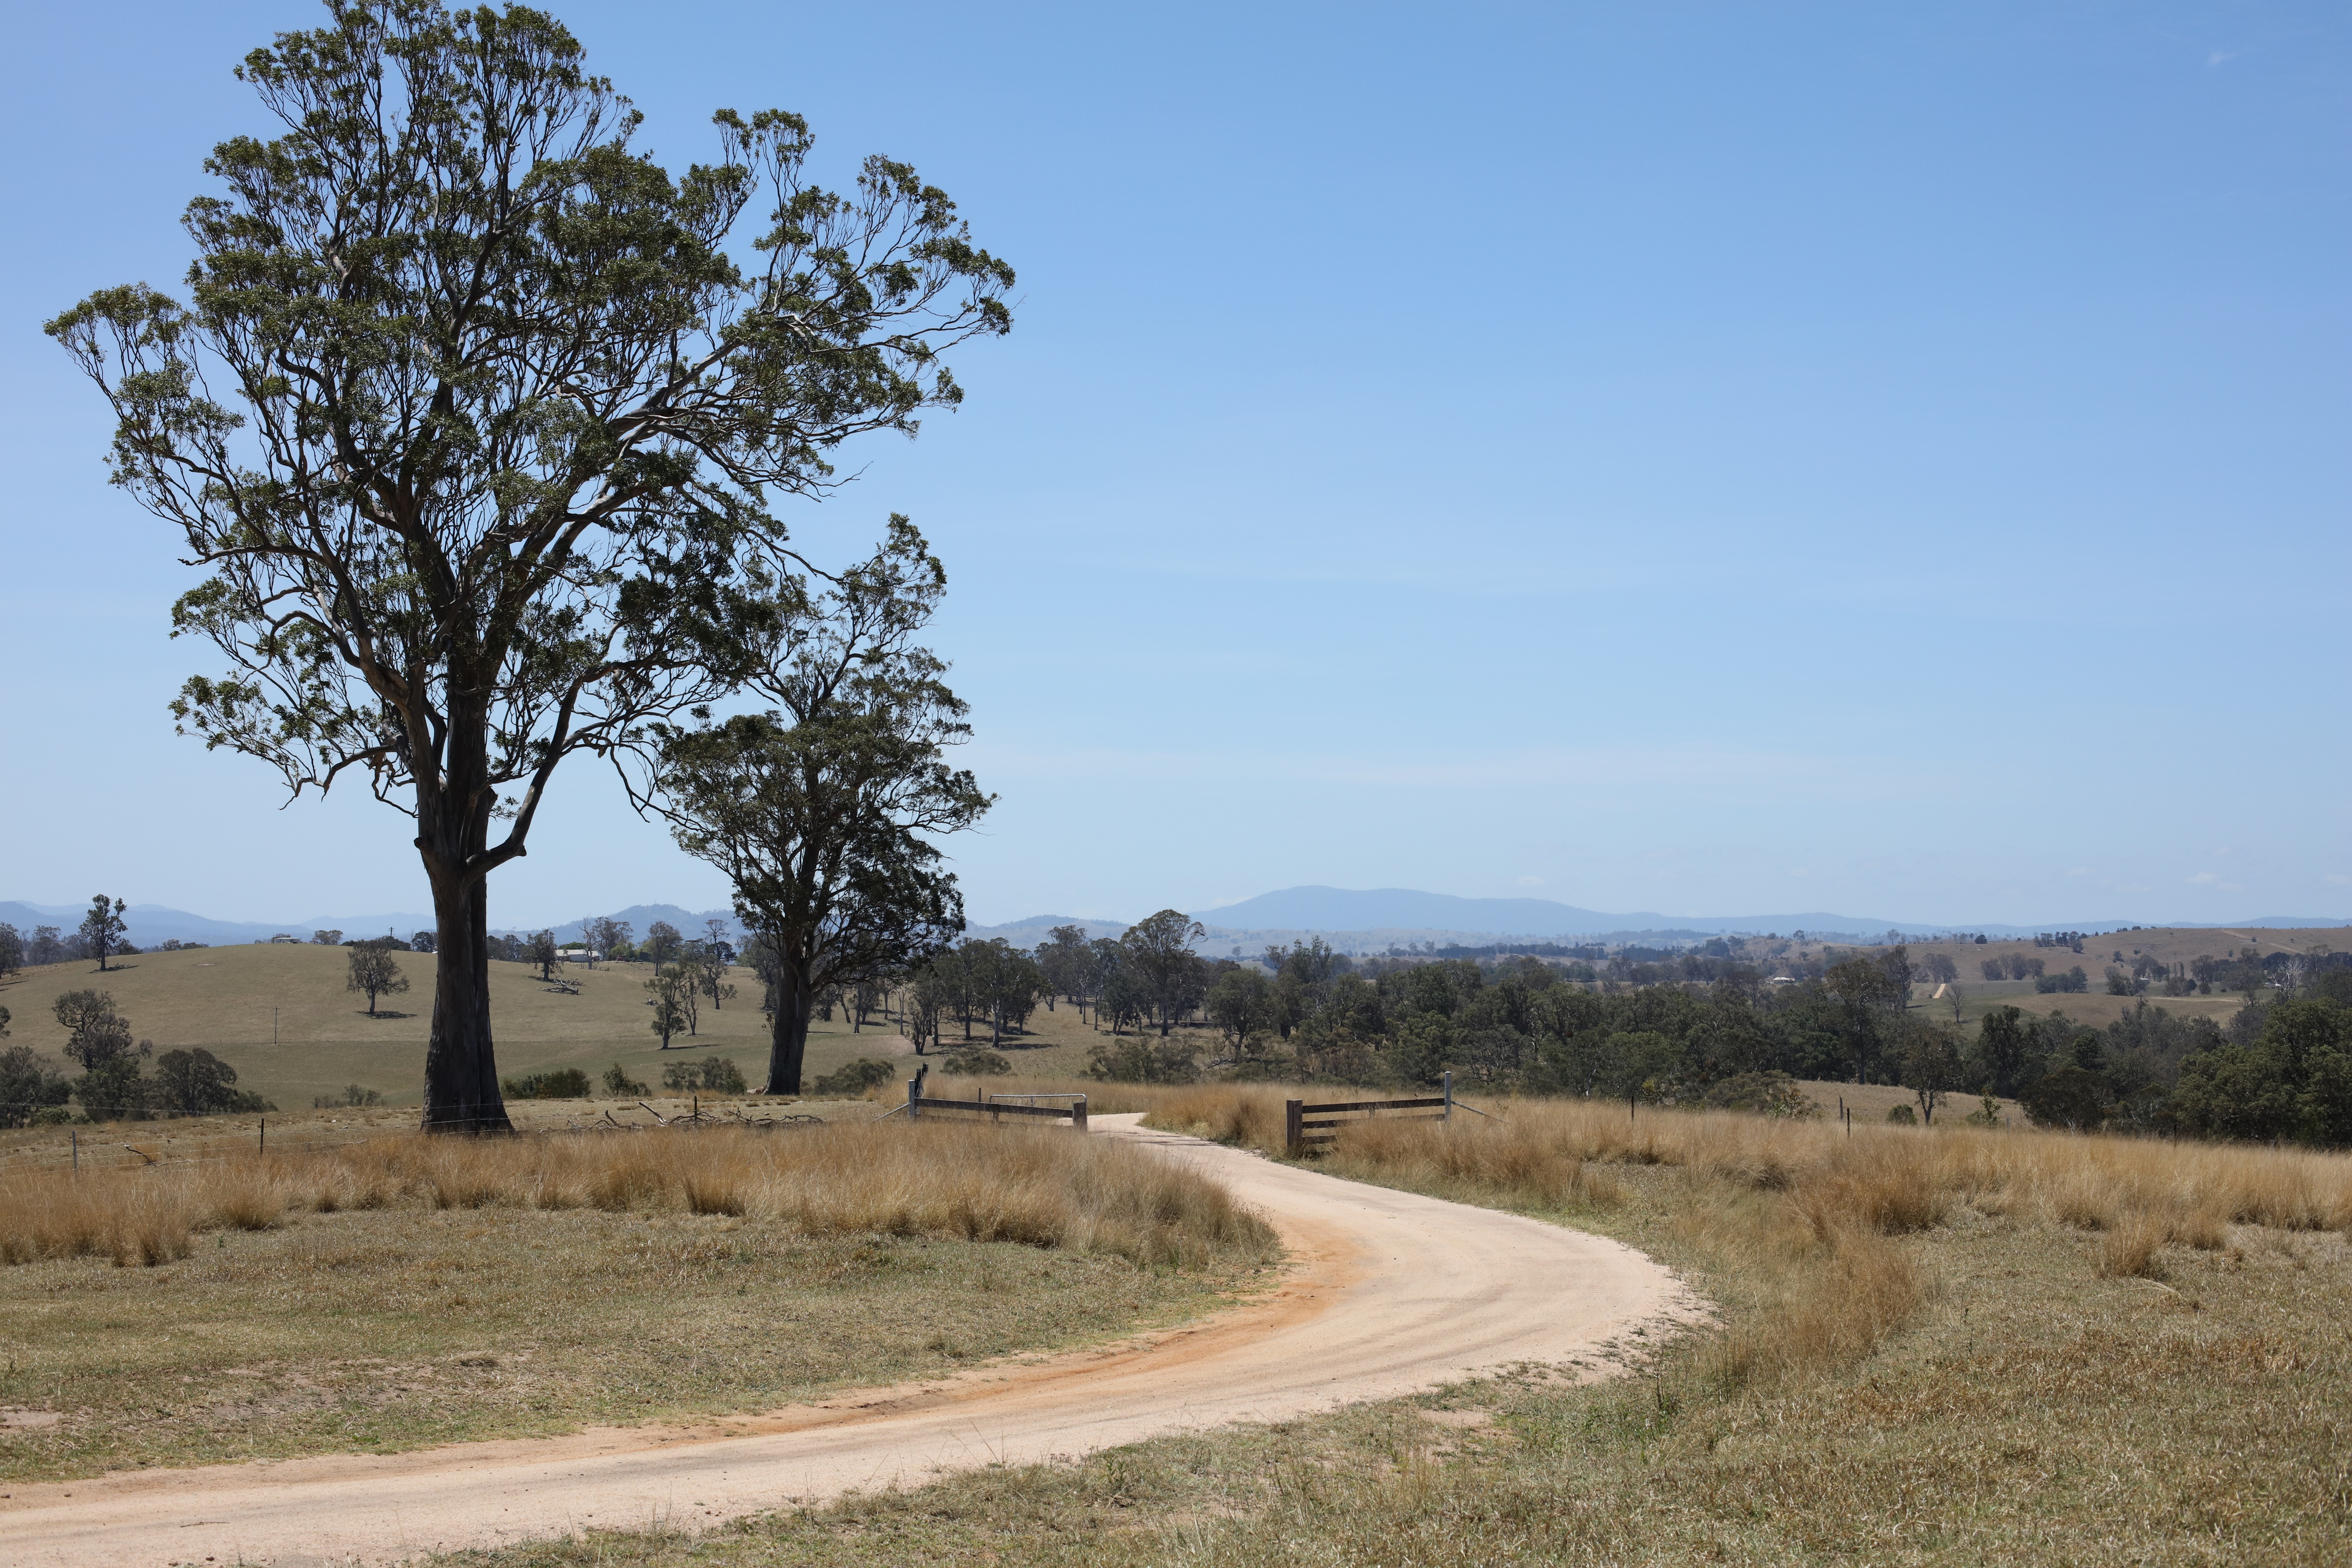}
    \label{fig:image3}
  \end{subfigure}
  \hfill
  \begin{subfigure}[b]{0.23\textwidth}
    \includegraphics[width=\textwidth]{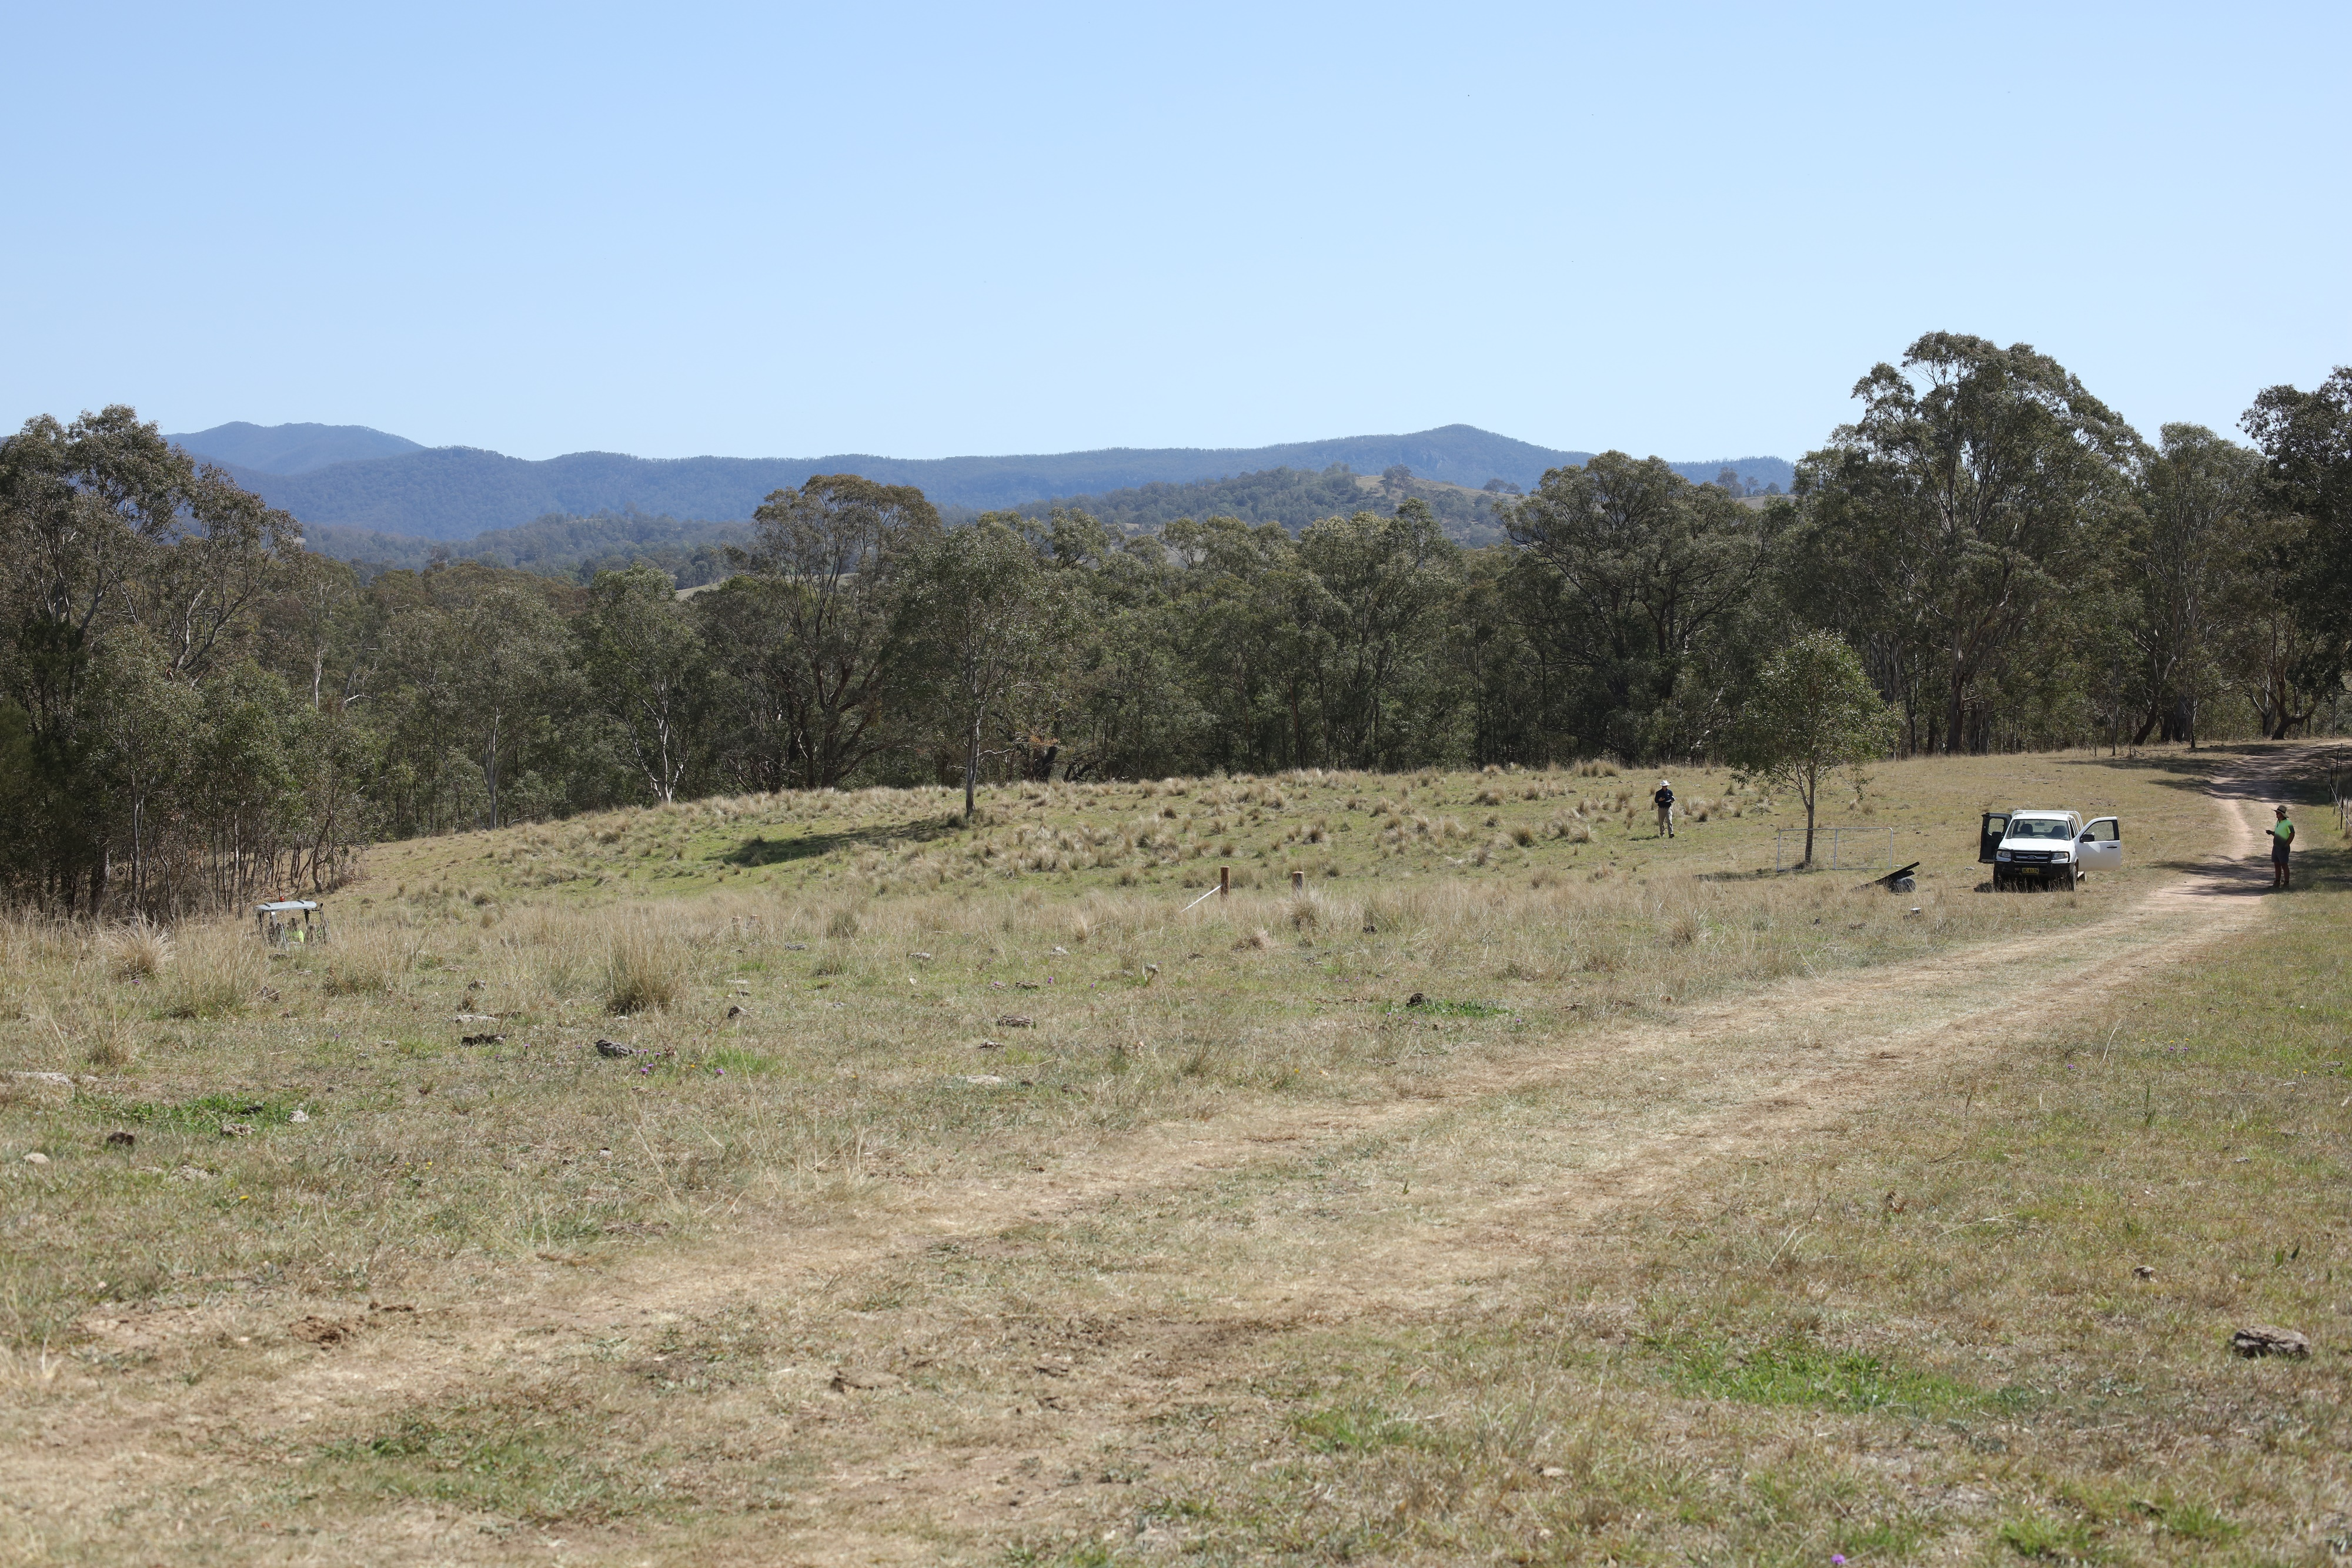}
    \label{fig:image4}
  \end{subfigure}
  \caption{Images depicting the research team in action, utilizing drone technology to capture diverse arrays of indigenous and invasive grass species in the Bega Valley, New South Wales, Australia. These efforts were critical in ensuring comprehensive coverage and high-quality data acquisition across different terrains and environmental conditions.}
  \label{fig:team_action}
\end{figure}
\section{Flight Parameters and Image Capture}
The drone flights were conducted at varying elevations—10m, 35m, and 120m above ground level (AGL)—to capture diverse perspectives of the surveyed area. Figures~\ref{fig:ch6/fr10}, \ref{fig:ch6/fr35}, and \ref{fig:ch6/fr120} illustrate sample images captured at these elevations, along with their corresponding binary masks indicating grass presence. The duration of each flight ranged from 5 to 20 minutes, depending on local wind conditions and the chosen elevation, with the pixel resolution at 10m elevation translating to approximately 0.2cm per pixel.

\begin{figure*}[!ht]
\centering
\begin{subfigure}[b]{0.32\textwidth}
  \centering
  \includegraphics[width=\linewidth,keepaspectratio]{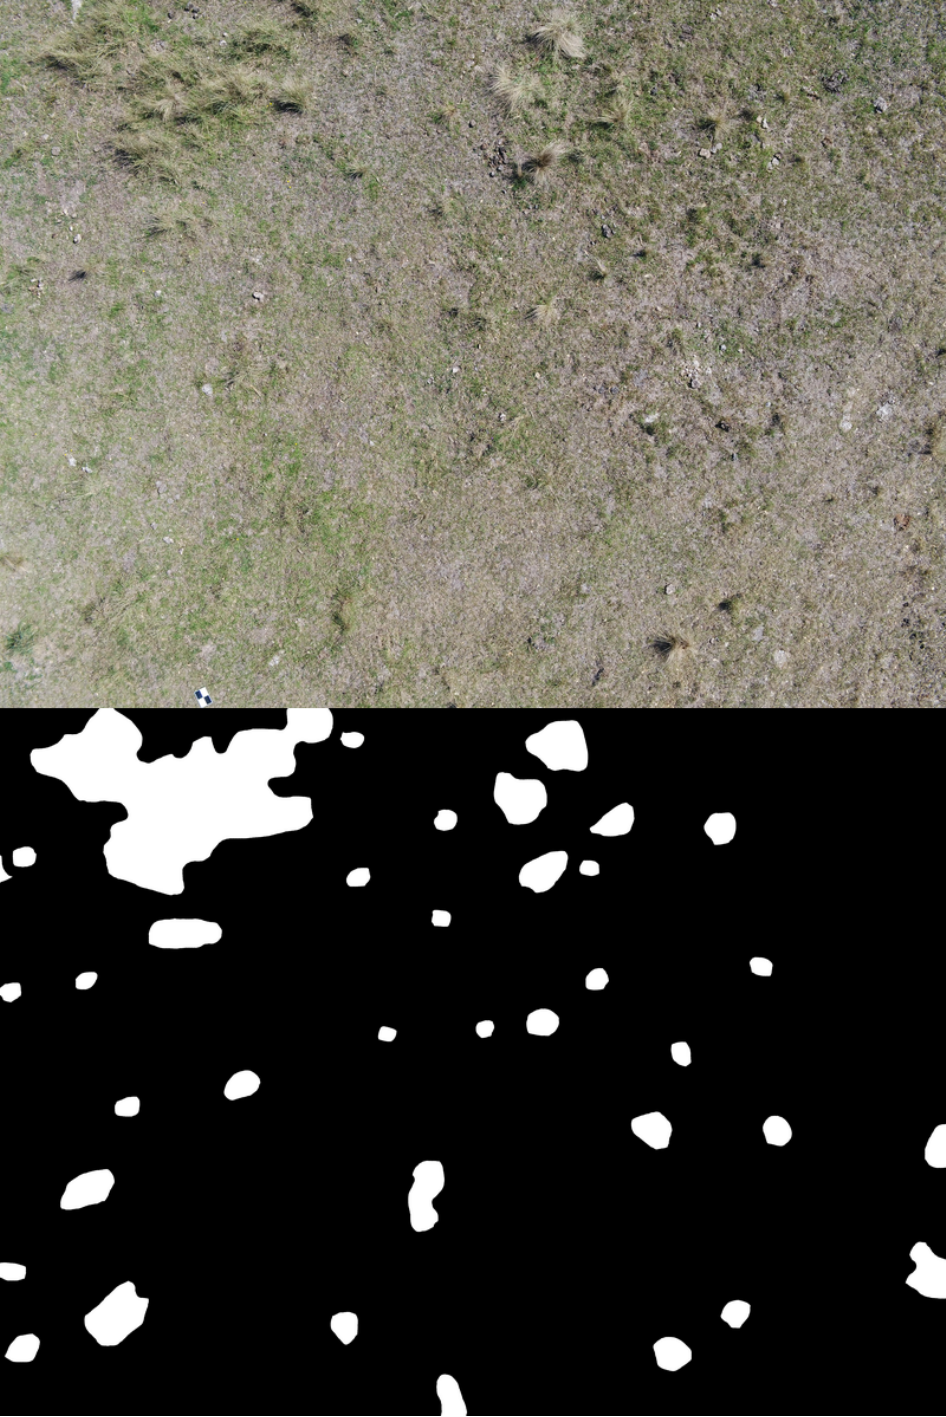}
  \caption{10m AGL}
  \label{fig:ch6/fr10}
\end{subfigure}
\hfill
\begin{subfigure}[b]{0.32\textwidth}
  \centering
  \includegraphics[width=\linewidth,keepaspectratio]{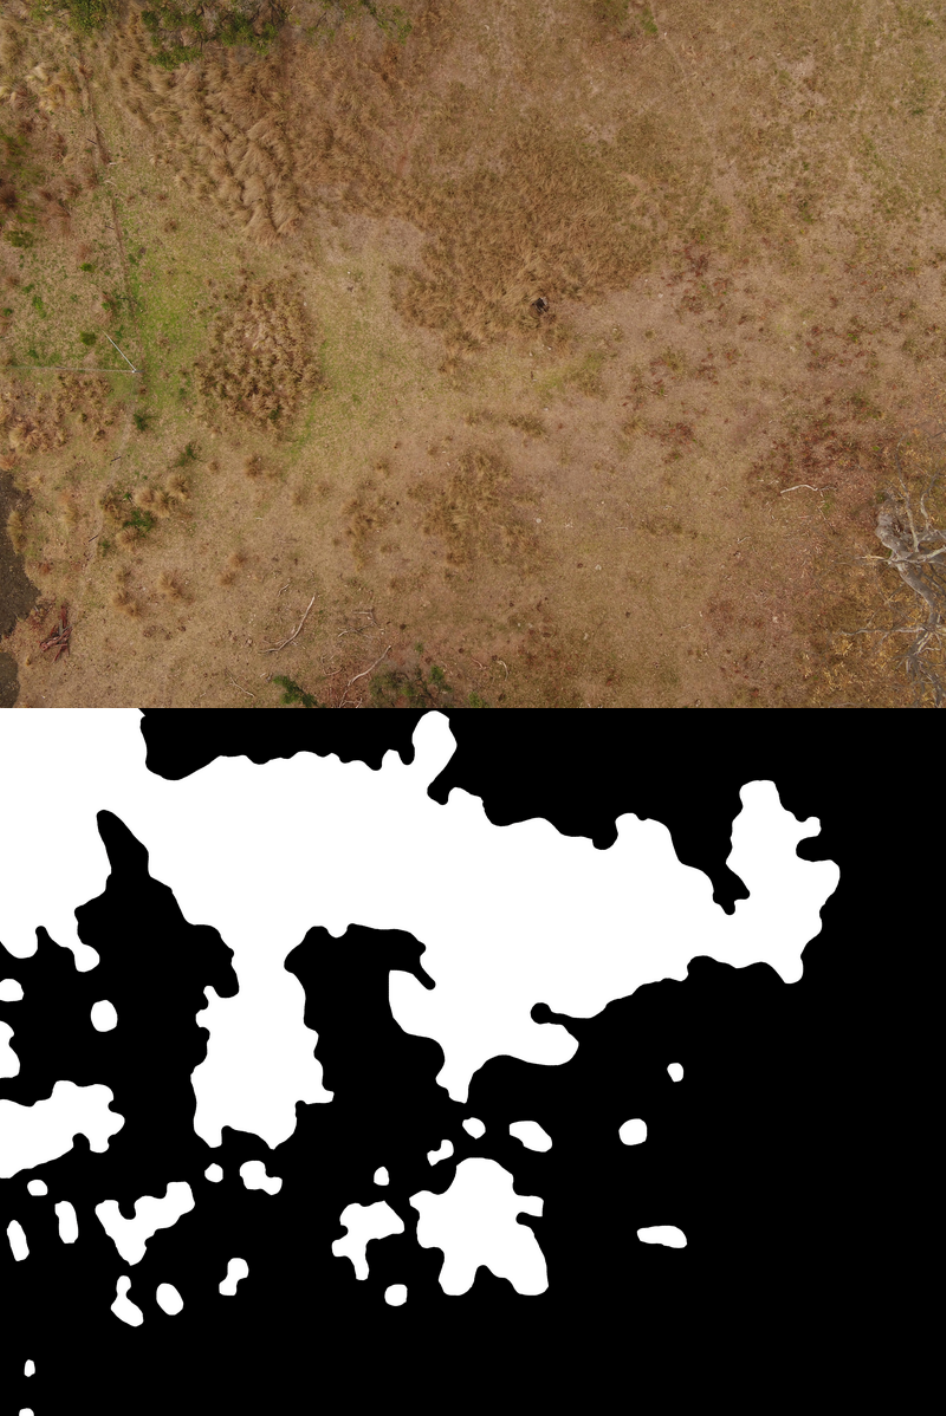}
  \caption{35m AGL}
  \label{fig:ch6/fr35}
\end{subfigure}
\hfill
\begin{subfigure}[b]{0.32\textwidth}
  \centering
  \includegraphics[width=\linewidth,keepaspectratio]{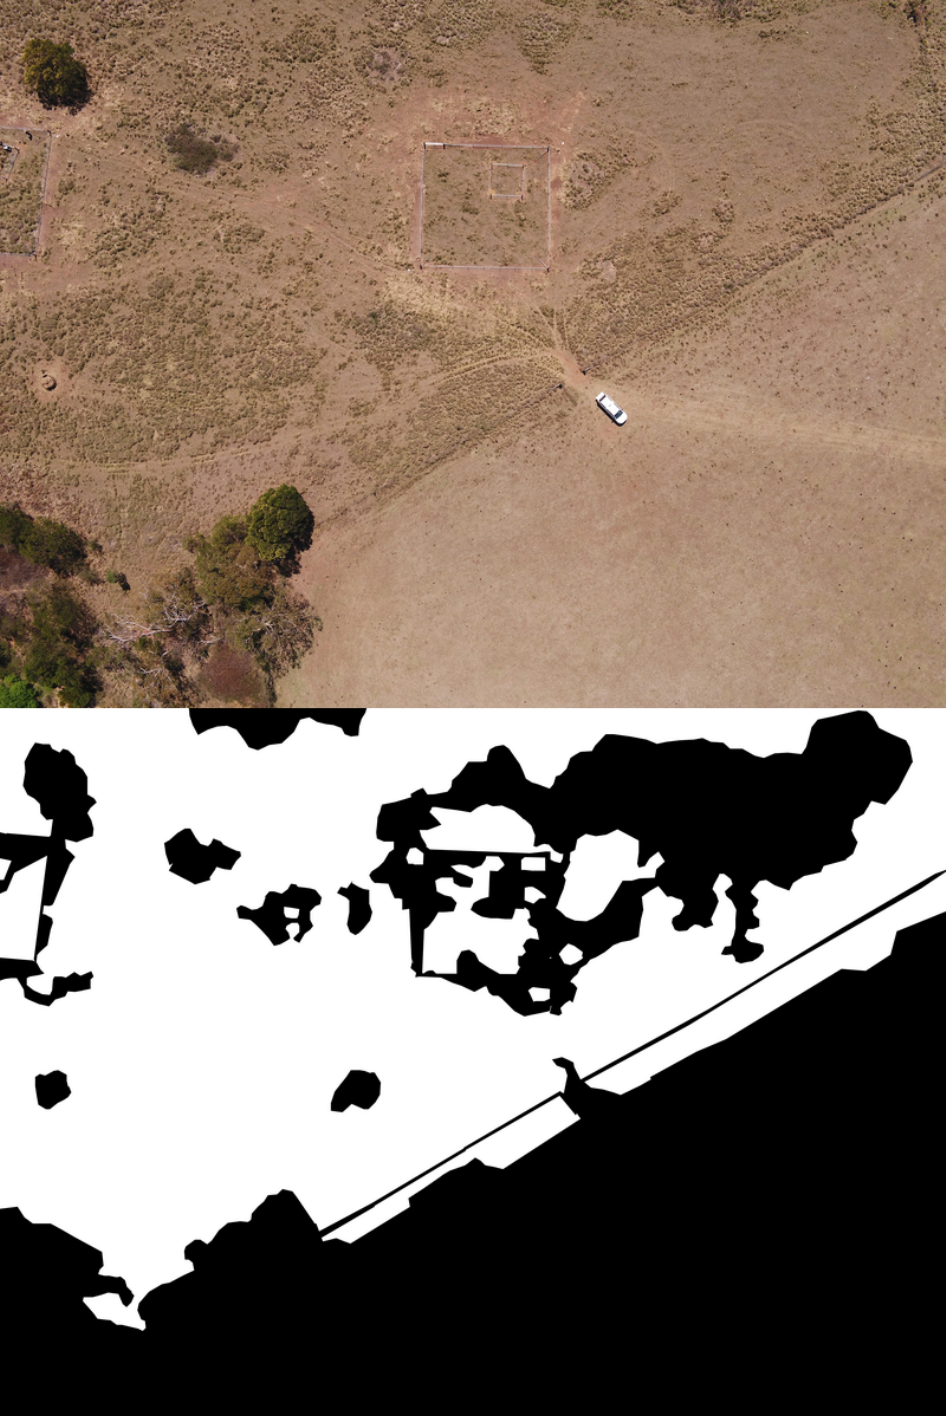}
  \caption{120m AGL}
  \label{fig:ch6/fr120}
\end{subfigure}
\caption{Images captured at varying elevations (AGL: Above Ground Level) with the DJI Inspire2, each accompanied by its binary mask. These illustrate the detail captured at 10m, 35m, and 120m AGL. The variation in elevation helps in understanding the impact of resolution on segmentation accuracy and the ability to detect fine-grained features of grass patches.}
\label{fig:ch6/fullres}
\end{figure*}

The use of multiple elevations allowed us to capture detailed imagery that supports robust segmentation model training. Lower elevations (10m AGL) provided high-resolution images crucial for identifying fine-grained features, while higher elevations (120m AGL) offered a broader view necessary for contextual understanding of the landscape.

\section{Data Collection Details}
Detailed data collection specifics, including dates, times, elevations, number of images, and white balance settings, are provided in Table~\ref{tbl:ch6/data}. This comprehensive data collection approach ensured a diverse and representative dataset, facilitating the development of models capable of generalizing across various conditions.

\begin{table*}[!ht]
\centering
\begin{threeparttable}
\caption{Data Collection Performed in Merimbula, NSW, Australia}
\setlength{\tabcolsep}{5pt} % Adjust the column spacing.
 % Adjust the row height.
\begin{tabular}{cccccc}
\toprule
\textbf{Date} & \textbf{Lot} & \textbf{Time} & \textbf{Elevation (AGL)} & \textbf{\# of Images} & \textbf{White Balance} \\ 
\midrule
2019-11-19 & L1a & 10:21-10:40 & 35m & 478 & Sunny \\
 &  & 11:02-11:10 & 120m & 113 & Sunny \\
 &  & 11:30-11:42 & 10m & 294 & Auto \\
 & L1b & 11:56-12:06 & 10m & 251 & Auto \\
 &  & 12:18-12:30 & 10m & 254 & Auto \\
 &  & 15:10-15:30 & 35m & 454 & Sunny \\
 &  & 15:42-15:48 & 120m & 113 & Sunny \\
 &  & 15:56-16:08 & 10m & 295 & Auto \\
 &  & 16:14-16:27 & 10m & 254 & Auto \\
2019-11-20 & L2a & 10:20-10:40 & 35m & 511 & Cloudy \\
 &  & 10:46-10:52 & 120m & 84 & Cloudy \\
 &  & 12:05-12:15 & 10m & 268 & Cloudy \\
 & L2b & 12:20-12:30 & 10m & 267 & Cloudy \\
 &  & 12:45-13:00 & 10m & 247 & Cloudy \\
 &  & 14:53-15:13 & 35m & 512 & Cloudy \\
 &  & 15:15-15:21 & 120m & 84 & Cloudy \\
 &  & 15:32-15:43 & 10m & 270 & Cloudy \\
 &  & 15:53-16:11 & 10m & 462 & Cloudy \\
2019-11-21 & L3 & 09:21-09:34 & 35m & 321 & Auto \\
 &  & 09:42-09:45 & 120m & 44 & Auto \\
 &  & 09:52-10:10 & 10m & 520 & Auto \\
\bottomrule
\end{tabular}
\begin{tablenotes}
\small
\item Note: Data collection details from Merimbula, NSW, Australia. Elevation is above ground level (AGL). White balance (WB) settings were adjusted based on prevailing lighting conditions.
\end{tablenotes}
\label{tbl:ch6/data}
\end{threeparttable}
\end{table*}

This detailed logging of flight parameters and conditions ensures transparency and reproducibility of our data collection process. The varying weather conditions and times of day captured in this dataset further contribute to its robustness and generalizability.

\section{Annotation Artifacts}
The annotation process implemented introduces several unique artifacts not commonly seen with other methodologies. One significant artifact arises from using a 64px circle brush for annotation. Specifically, this brush size tends to produce inaccuracies around edges with concave angles, such as the spaces between blades of grass. The larger the brush, the more pronounced the error, particularly around sharp angles. For instance, at an elevation of 10 meters, the worst-case scenario using a 64px brush could lead to an area error of approximately 12.8 square centimeters, with this error magnitude linearly increasing at higher elevations.

Another related issue occurs when annotating non-grass sections smaller than 64px (or roughly 12.8cm²). In these cases, the annotation typically defaults to a single brush-sized circle on the targeted grass patch, as illustrated in Fig.~\ref{fig:ch6/da}. These types of inaccuracies are absent when employing a 1px brush, assuming the annotator makes no mistakes—a presumption that's not practical.

\begin{figure*}[!ht]
\centering
\begin{subfigure}[b]{0.32\textwidth}
  \centering
  \fbox{\includegraphics[width=\linewidth]{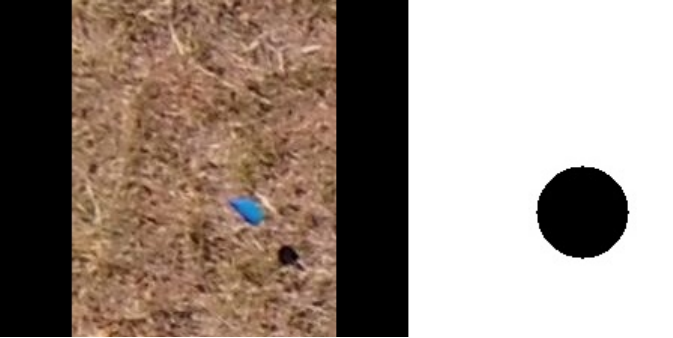}}
  \caption{}
  \label{fig:ch6/da1}
\end{subfigure}
\hfill
\begin{subfigure}[b]{0.32\textwidth}
  \centering
  \fbox{\includegraphics[width=\linewidth]{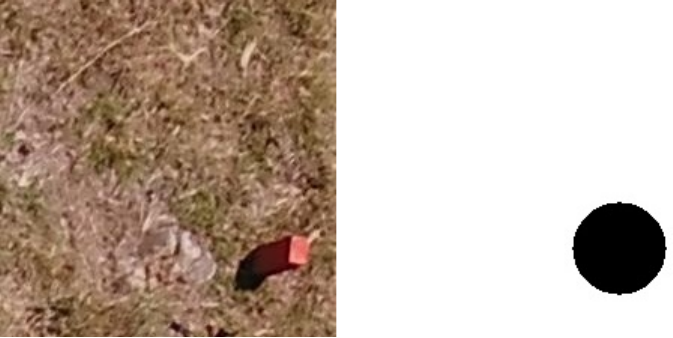}}
  \caption{}
  \label{fig:ch6/da2}
\end{subfigure}
\hfill
\begin{subfigure}[b]{0.32\textwidth}
  \centering
  \fbox{\includegraphics[width=\linewidth]{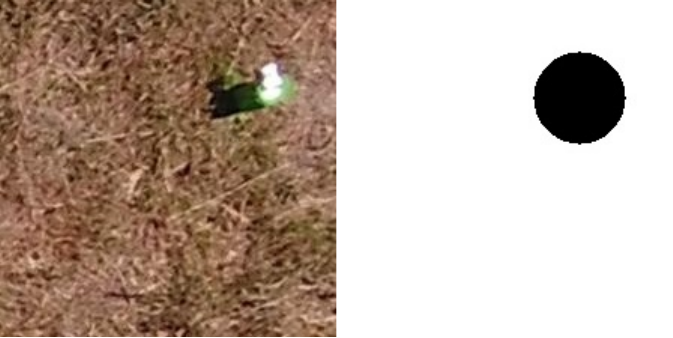}}
  \caption{}
  \label{fig:ch6/da3}
\end{subfigure}
\vspace{-1ex}
\caption{Three examples of artifacts resulting from the use of a 64px circle brush for annotation. These artifacts highlight the challenges in achieving precise annotations, particularly around fine and intricate structures like grass blades.}
\label{fig:ch6/da}
\end{figure*}

Additionally, the methodology restricts viewing the image at magnifications beyond 100\%, limiting the annotator’s ability to perform highly precise, pixel-wise annotations. While it reduces one type of error, this constraint potentially introduces others, such as perceiving pixels as mere color patches rather than distinct features like individual blades of grass.

A noteworthy artifact emerges in the presence of fence-lines, as depicted in Fig.~\ref{fig:ch6/fa}. The fence-lines create complex scenarios where grass exists along and through the fence-line, leading to artifacts resembling long brush strokes appearing amidst the grass. This phenomenon, like the others mentioned, stems from the limitations and characteristics of the chosen annotation tools and settings.

\begin{figure*}[!ht]
\centering
\begin{subfigure}[b]{0.32\textwidth}
  \centering
  \fbox{\includegraphics[width=\linewidth]{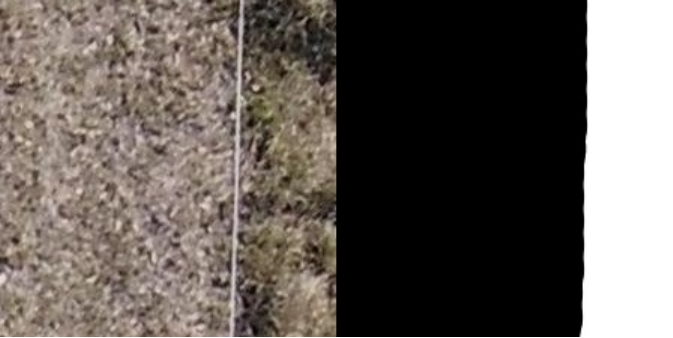}}
  \caption{}
  \label{fig:ch6/fa1}
\end{subfigure}
\hfill
\begin{subfigure}[b]{0.32\textwidth}
  \centering
  \fbox{\includegraphics[width=\linewidth]{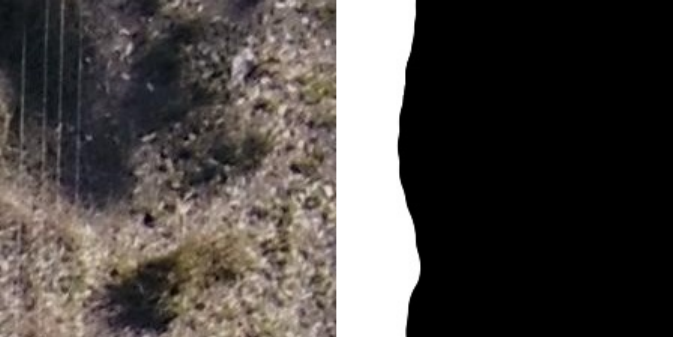}}
  \caption{}
  \label{fig:ch6/fa2}
\end{subfigure}
\hfill
\begin{subfigure}[b]{0.32\textwidth}
  \centering
  \fbox{\includegraphics[width=\linewidth]{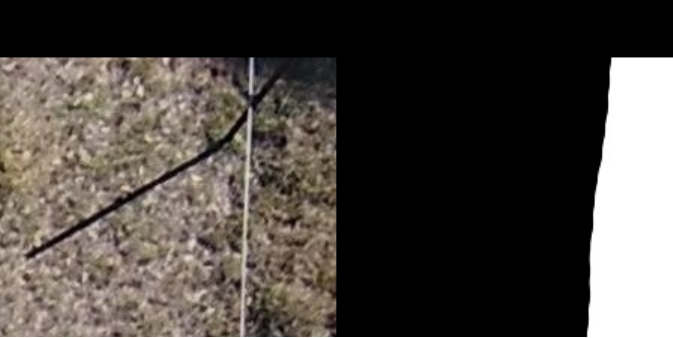}}
  \caption{}
  \label{fig:ch6/fa3}
\end{subfigure}
\vspace{-1ex}
\caption{Three examples of an artifact that occurs along fence-lines due to ambiguity in distinguishing between fence-line and grass. These artifacts pose significant challenges for segmentation models, necessitating advanced techniques to improve accuracy.}
\label{fig:ch6/fa}
\end{figure*}
